# Supplementary material for: A City of Millions: Mapping Literary Social Networks At Scale
Source: arXiv:2502.19590 source file (2025-03-28)
Supplement: Supplementary file 1 [file appendix.tex]

\onecolumn
\small
\section{Model Prompt}
\label{sec:modelPrompt}
\begin{verbatim}
def get_prompt(text): 
    js = """*Output Format*:
    [begin format]
    Please provide your response with the following
    JSON schema: 
    {
        "$schema": "http://json-schema.org/draft-07/
            schema#",
        "type": "object",
        "title": "Character Relationship Schema",
        "description": "Schema for describing 
            relationships between literary characters",
        "required": [
            "character_1",
            "character_2",
            "affinity",
            "coarse_category",
            "fine_category"
        ],
        "properties": {
            "character_1": {
                "type": "string",
                "description": "First character in the relationship"
            },
            "character_2": {
                "type": "string",
                "description": "Second character in the relationship"
            },
            "affinity": {
                "type": "string",
                "enum": ["positive", "negative", "neutral"],
                "description": "The nature of the relationship between characters"
            },
            "coarse_category": {
                "type": "string",
                "enum": ["professional", "social", "social"],
                "description": "Broad category of the relationship"
            },
            "fine_category": {
                "type": "string",
                "description": "Specific type of relationship",
                "enum": [
                    "friend",
                    "enemy",
                    "acquaintance",
                    "lovers",
                    "unrequited love interest",
                    "rivals",
                    "employer",
                    "employee",
                    "colleague",
                    "servant",
                    "master",
                    "student",
                    "teacher",
                    "client",
                    "person offering service to client",
                    "husband",
                    "wife",
                    "brother",
                    "sister",
                    "cousin",
                    "uncle",
                    "aunt",
                    "niece",
                    "nephew",
                    "child",
                    "parent",
                    "grandchild",
                    "grandparent",
                    "orphan",
                    "foster parent",
                    "step-child",
                    "step-parent",
                    "in-law relation",
                    "half relation"
                ]
            },
        },
        "additionalProperties": false
    }
    [end format]
    
    *Example output for Don Quixote*:
    [begin example]
    [
        {
            "character_1": "Sancho Panza",
            "character_2": "Don Quixote",
            "affinity": "neutral",
            "coarse_category": "professional",
            "fine_category": "employer"
        },
        {
            "character_1": "Rocinante",
            "character_2": "Don Quixote",
            "affinity": "positive",
            "coarse_category": "professional",
            "fine_category": "friend"
        },
        {
            "character_1": "Dulcinea del Toboso",
            "character_2": "Don Quixote",
            "affinity": "neutral",
            "coarse_category": "social",
            "fine_category": "unrequited love interest"
        },
        {
            "character_1": "Cervantes",
            "character_2": "Cide Hamete Benengeli",
            "affinity": "positive",
            "coarse_category": "professional",
            "fine_category": "colleague"
        },
        {
            "character_1": "The Duke and Duchess",
            "character_2": "Don Quixote",
            "affinity": "neutral",
            "coarse_category": "social",
            "fine_category": "enemy"
        },
        {
            "character_1": "The Duke and Duchess",
            "character_2": "Sancho Panza",
            "affinity": "neutral",
            "coarse_category": "social",
            "fine_category": "enemy"
        },
        {
            "character_1": "Don Quixote",
            "character_2": "Altisidora",
            "affinity": "negative",
            "coarse_category": "social",
            "fine_category": "lovers"
        },
        {
            "character_1": "Altisidora",
            "character_2": "The Duke and Duchess",
            "affinity": "neutral",
            "coarse_category": "professional",
            "fine_category": "employee"
        },
        {
            "character_1": "The priest",
            "character_2": "Don Quixote",
            "affinity": "positive",
            "coarse_category": "social",
            "fine_category": "friend"
        },
        {
            "character_1": "Sampson Carrasco",
            "character_2": "Don Quixote",
            "affinity": "negative",
            "coarse_category": "social",
            "fine_category": "enemy"
        },
        {
            "character_1": "Sancho Panza",
            "character_2": "Dapple",
            "affinity": "neutral",
            "coarse_category": "social",
            "fine_category": "friend"
        },
        {
            "character_1": "The barber",
            "character_2": "Don Quixote",
            "affinity": "positive",
            "coarse_category": "social",
            "fine_category": "friend"
        }
    ]
    [end example]
    """
    return f"""*text*:
    [begin text]
    {text}
    [end text]
    
    *task*:
    [begin task]
    In this task, you’ll be identifying the relationship types that exists between pairs of 
    characters in the above text, using the whole text as provided. (For example, if reading 
    To Kill a Mockingbird, you’d mark that Atticus Finch is the father of Scout Finch.)
    
    After reading the text, answer the following questions for pairs of characters using these 
    guidelines:
    [end task]
    
    *Target*:
    [begin characters]
    Only produce a single annotation per character pair.
    [end characters]
    
    *Affinity*:
    [begin affinity]
    How do the two characters feel toward each other? For example, if they are friendly, select 
    "Positive". If it is unclear how they feel toward each other or if they do not have strong 
    opinions about each other, select "Neutral". If they are enemies or rivals, or hate each 
    other, select "Negative".
    [end affinity]
    
    *Category*:
    [begin category]
    How are the two characters related? If they are friends, say "Social". If they share a
    relationship because they work with each other, say "Professional". If they 
    are family, then say "Familial".
    [end category]
    
    *Kind*:
    [begin kind]
    Specifically, how is the First Character related to the Second Character? For example,
    if the First Character is the husband of the Second Character, then select "husband". Please 
    keep the Category and the Kind consistent:
    
    If you say "Social", then the Kind must be one of these:
        • friend
        • enemy
        • acquaintance
        • lovers
        • unrequited love interest (X is in love with Y, but Y is not in love with X)
        • rivals
    
    If you say "Professional", then the Kind must be one of these:
        • employer
        • employee
        • colleague
        • servant
        • master
        • student
        • teacher
        • client
        • person offering service to client (e.g., lawyer)
        
    If you say "Familial", then the Kind must be one of these:
        • husband/wife
        • brother/sister
        • cousin
        • uncle/aunt
        • niece/nephew
        • child
        • parent
        • grandchild
        • grandparent
        • orphan
        • foster parent
        • step-child
        • step-parent
        • in-law relation (e.g., mother-in-law; specify in detail)
        • half relation (e.g., half-sister; specify in detail)
    [end kind]
    {js}
    Begin the task!
    """
\end{verbatim}
